# Supplementary material for: Multivariate longitudinal modeling of cross-sectional and lagged associations between a continuous time-varying endogenous covariate and a non-Gaussian outcome
Source: arXiv:2511.11114 source file (2025-11-14)
Supplement: Supplementary file 1 [file main.tex]

\documentclass{article}

% Language setting
% Replace `english' with e.g. `spanish' to change the document language
\usepackage[english]{babel}

% Set page size and margins
% Replace `letterpaper' with `a4paper' for UK/EU standard size
\usepackage[letterpaper,top=2cm,bottom=2cm,left=3cm,right=3cm,marginparwidth=1.75cm]{geometry}
\usepackage{algorithm}
\usepackage{algpseudocode}

% Useful packages
\usepackage{amsmath}
\usepackage{graphicx}
\usepackage[labelfont=bf]{caption}  % Only "Figure X" is bold
\usepackage{mathtools}
\usepackage{xcolor}
\usepackage[colorlinks=true, allcolors=blue]{hyperref}
\usepackage{subcaption}
\usepackage{authblk}

\title{\Large{\textbf{
Multivariate longitudinal modeling with continuous time-varying endogenous covariates - Supplementary material
}}}
\author[1]{Chiara Degan}
\author[1]{Bart J.A. Mertens}
\author[1]{Jelle Goeman}
\author[2]{Nadine A. Ikelaar}
\author[2]{Erik H. Niks}
\author[3]{Pietro Spitali}
\author[1]{Roula Tsonaka}
\affil[1]{Department of Biomedical Data Sciences, Leiden University Medical Center, The Netherlands}
\affil[2]{Department of Neurology, Leiden University Medical Center, The Netherlands}
\affil[3]{Department of Human Genetics, Leiden University Medical Center, The Netherlands}
\date{}

\begin{document}
\maketitle

\section{Association coefficient}
This section provides a detailed derivation of the association coefficient, as introduced in Section 3.2 of the paper, with a distinction made between the two joint models: JMM and JSM.\\
For details about the notation, refer to Section 3 of the paper.

\subsection{Joint Mixed Model}\label{JMM supp}
\subsubsection{General case}
Let's assume one continuous endogenous variable $\mathbf{v}_i$ and one non-continuous response variable $\mathbf{y}_i$:
\begin{equation*}
\label{JMM equation}
\left\{\begin{aligned}
& \mathbf{v}_i = \mathbf{X}^{\text{v}}_i\boldsymbol{\beta}^\text{v} + \mathbf{Z}^{\text{v}}_i\mathbf{b}^{\text{v}}_i+\boldsymbol{\varepsilon}_i \\
& g(\boldsymbol{\mu}_i) = \boldsymbol{\eta}_i = \mathbf{X}^{\text{y}}_i\boldsymbol{\beta}^\text{y} + \mathbf{Z}^{\text{y}}_i\mathbf{b}^{\text{y}}_i
\end{aligned}\right.
\qquad \qquad \boldsymbol{\varepsilon}_i \sim \mathcal{N} (\mathbf{0}, \mathbf{\Sigma}_i = \sigma^{2}\textbf{I}_{n_i})
\end{equation*}
where the random effects of the two variables are normally distributed
\begin{equation*}
\mathbf{b}_i^{\text{v}} \sim \mathcal{N} \left(
\mathbf{0}, \mathbf{D}_{\text{v}} \right) \qquad
\mathbf{b}_i^{\text{y}} \sim \mathcal{N} \left(
\mathbf{0}, 
\mathbf{D}_{\text{y}}
\right)  
\end{equation*}
and correlated
\begin{equation*}
\label{eq:random effects}
\mathbf{b}_{i} =
\left[\begin{array}{l}
\mathbf{b}^{\text{v}}_{i} \\
\mathbf{b}^{\text{y}}_{i}
\end{array}\right] \sim \mathcal{N}\left(\boldsymbol{\mu}_{\text{b}} = \mathbf{0}, \mathbf{D} =\left[\begin{array}{ll}
\mathbf{D}_{\text{v}} & \mathbf{D}_{\text{vy}} \\
\mathbf{D}_{\text{yv}} & \mathbf{D}_{\text{y}}
\end{array}\right]\right).
\end{equation*}
Refer to the manuscript for a more detailed explanation about the Joint Mixed Model structure.\\
Based on the theory of the Mixed Effects Models we know that the marginal distribution of the endogenous variable is:
\begin{align*}
& \mathbf{v}_i \sim \mathcal{N}_{n_i} \left(\boldsymbol{\mu}_\text{v} = \mathbf{X}^{\text{v}}_i\boldsymbol{\beta}^\text{v}, \text{var}(\mathbf{v}_i) = \mathbf{Z}^{\text{v}}_i\mathbf{D}_{\text{v}}\mathbf{Z}_i^{\text{v}\top}+\mathbf{\Sigma}_i\right).
\end{align*}\\ \\
The integral that we want to solve in order to derive the marginal association coefficient is:
\begin{equation}
\label{ass jmm}
\begin{aligned}
E\left[y_{ik} \mid v_{ij} = a\right] 
& =\int_y y_{i k} f\left(y_{i k} \mid v_{i j}=a\right) \; d y_{ik}  \\
& = \int_y y_{i k} \; \frac{f\left(y_{i k}, v_{i j}=a\right)}{f(v_{i j}=a)} \; d y_{ik} \\
& = \int_y y_{i k} \; \frac{f\left(y_{i k}, v_{i j}=a \mid \mathbf{b}_i \right) f(\mathbf{b}_i)}{f(v_{i j}=a)} \; d y_{ik}  \\ 
& = \int_y y_{i k} \int_b \frac{f(y_{i k} \mid \mathbf{b}_i)f(v_{i j}=a \mid \mathbf{b}_i) f(\mathbf{b}_i) }{f(v_{i j}=a)} \; d \mathbf{b}_i \, d y_{ik}  \\ 
& = \int_y \int_b y_{i k} f\left(y_{i k}\mid \mathbf{b}_i\right)\; \frac{ f(v_{i j}=a \mid \mathbf{b}_i) f(\mathbf{b}_i) }{f(v_{i j}=a)} \; d \mathbf{b}_i \, d y_{ik}  \\ 
& = \int_b \textcolor{red}{\int_y y_{i k} f\left(y_{i k} \mid \mathbf{b}_i\right)} \textcolor{blue}{f\left(\mathbf{b}_i \mid v_{i j}=a\right)} \; \textcolor{red}{d y_{ik}} \, d \mathbf{b}_i.
\end{aligned}
\end{equation}
Since $\mathbf{y}_i$ and $\mathbf{v}_i$
are of different types, their joint distribution form is unknown. \\
We assume that the association between these two variables is fully captured by the correlation of the random effects. Under this assumption, $\mathbf{y}_i$ and $\mathbf{v}_i$
are conditionally independent given the random effects. This conditional independence allows the distribution $f\left(y_{i k}, v_{i j}=a \mid \mathbf{b}_i \right)$ to be factorized into the product $f(y_{i k} \mid \mathbf{b}_i)f(v_{i j}=a \mid \mathbf{b}_i)$ (as seen in the transition from the third to the fourth row).\\
\\
We know the first part of the integral being the mean of $y_{ik}$ conditional on the random effects $\mathbf{b}_i$:
\begin{equation}
\label{cond mean jmm}
\textcolor{red}{\int_y y_{i k} f\left(y_{i k} \mid \mathbf{b}_i\right)\; d y_{ik} = g^{-1}(\eta_{ik})}.
\end{equation}
We also know the second part of integral (\ref{ass jmm}). $\mathbf{v}_i$ and $\mathbf{b}_i$ are both normally distributed, so their joint and conditional distributions are automatically Gaussian:
$$f(\mathbf{b}_i, \mathbf{v}_i) \sim \mathcal{N} \left( \boldsymbol{\mu} = \left[\begin{array}{l}
\boldsymbol{\mu}_\text{b}\\
\boldsymbol{\mu}_\text{v}
\end{array}\right], \mathbf{\Omega} = \left[\begin{array}{ll}
\mathbf{D} & \mathbf{\Omega}_{\text{bv}}\\
\mathbf{\Omega}_{\text{bv}} &  \text{var}(\mathbf{v}_i)
\end{array}\right]
\right),$$ 
\begin{equation}
\label{cond b}
    \textcolor{blue}{f(\mathbf{b}_i\mid \mathbf{v}_{i} = \mathbf{a}) \sim \mathcal{N} \left(\boldsymbol{\mu}_\text{b} + \mathbf{\Omega}_{\text{bv}}  \text{var}(\mathbf{v}_{i})^{-1}(\mathbf{a} - \boldsymbol{\mu}_\text{v}), \mathbf{D} - \mathbf{\Omega}_{\text{bv}}  \text{var}(\mathbf{v}_{i})^{-1} \mathbf{\Omega}_{\text{bv}}\right)}
\end{equation}

\subsubsection{Normal case}\label{normal subsection jmm}
Let's assume the same model as before but with an identity link function:
\begin{equation*}
\left\{\begin{aligned}
& \mathbf{v}_i = \mathbf{X}^{\text{v}}_i\boldsymbol{\beta}^\text{v} + \mathbf{Z}^{\text{v}}_i\mathbf{b}^{\text{v}}_i+\boldsymbol{\varepsilon}^{\text{v}}_i \\
& \mathbf{y}_i = \mathbf{X}^{\text{y}}_i\boldsymbol{\beta}^\text{y} + \mathbf{Z}^{\text{y}}_i\mathbf{b}^{\text{y}}_i + \boldsymbol{\varepsilon}^{\text{y}}_i
\end{aligned}\right.
\qquad \qquad \begin{aligned}
\boldsymbol{\varepsilon}^{\text{v}}_i \sim \mathcal{N} (\mathbf{0}, \mathbf{\Sigma}^\text{v}_i = \sigma_v^{2}\textbf{I}_{n_i})\\
\boldsymbol{\varepsilon}^{\text{y}}_i \sim \mathcal{N} (\mathbf{0}, \mathbf{\Sigma}^\text{y}_i = \sigma_\text{y}^{2}\textbf{I}_{m_i})
\end{aligned}
\end{equation*}
In this case $E\left[y_{ik} \mid v_{ij} = a\right]$ can be define by a closed formula. To derive it we need to define first the joint distribution of $\mathbf{y}_i$ and $\mathbf{v}_i$. The joint distribution is a bivariate Gaussian:
$$
f\left(\mathbf{y}_i, \mathbf{v}_i\right)=\mathcal{N}_2\left(\left[\begin{array}{l}
\boldsymbol{\mu}_{\text{y}} \\
\boldsymbol{\mu}_{\text{v}}
\end{array}\right],\left[\begin{array}{cc}
\text{var}(\mathbf{y}_i) & \text{cov}(\mathbf{y}_i, \mathbf{v}_i) \\
\text{cov}(\mathbf{y}_i, \mathbf{v}_i) & \text{var}(\mathbf{v}_i) 
\end{array}\right]\right) 
$$
From the bivariate normal, the conditional distribution of the response variable $y_{ik}$ given the time-varying covariate $v_{ij}$ can be simply derived:
$$
f\left(y_{ik} \mid v_{ij} = a\right)=\mathcal{N}\left(\mu^{\text{y}}_{ik}+\frac{\text{cov}(y_{ik}, v_{ij})}{\text{var}(v_{ij})}\left(a-\mu^{\text{v}}_{ij}\right),\text{var}(y_{ik}) - \frac{\text{cov}(y_{ik}, v_{ij})^2}{\text{var}(v_{ij})}\right).
$$\\
Then the association coefficient $\beta_{joint}$ is defined as:
\begin{equation}
\label{ass jmm normal}
\begin{aligned}
& E\left[y_{ik} \mid v_{ij} = a + 1\right]-E\left[y_{ik} \mid v_{ij} = a\right]= \\
&=\left(\mu^{\text{y}}_{ik}+\frac{\text{cov}(y_{ik}, v_{ij})}{\text{var}(v_{ij})}\left(a+1-\mu^{\text{v}}_{ij}\right)\right)-\left(\mu^{\text{y}}_{ik}+\frac{\text{cov}(y_{ik}, v_{ij})}{\text{var}(v_{ij})}\left(a-\mu^{\text{v}}_{ij}\right)\right)= \\
&=\frac{\text{cov}(y_{ik}, v_{ij})}{\text{var}(v_{ij})} .
\end{aligned}
\end{equation}
\subsection{Joint Scaled Model}\label{JSM supp}
\subsubsection{General case}
Let's assume one continuous endogenous variable $\mathbf{v}_i$ and one non-continuous response variable $\mathbf{y}_i$:
\begin{equation*}
\label{JSM eq}
\left\{\begin{aligned}
& \mathbf{v}_i=\mathbf{m}_i+\boldsymbol{\varepsilon}_{i} \\
& \mathbf{m}_i = \mathbf{X}^{\text{v}}_{i} \boldsymbol{\beta}^{\text{v}}+\mathbf{Z}^{\text{v}}_{i} \mathbf{b}^{\text{v}}_{i} \\
& g(\boldsymbol{\mu}_i) = \boldsymbol{\eta}_i = \mathbf{X}^{\text{y}}_i\boldsymbol{\beta}^\text{y} + \mathbf{Z}^{\text{y}}_i\mathbf{b}^{\text{y}}_i + \gamma \mathbf{m}_i
\end{aligned}\right.
\end{equation*}
Refer to the manuscript for a more detailed explanation about the Joint Scaled Model structure.\\
Based on the theory of the Mixed Effects Models we know that the marginal distribution of the endogenous variable is:
\begin{align*}
& \mathbf{v}_i \sim \mathcal{N}_{n_i} \left(\boldsymbol{\mu}_\text{v} = \mathbf{X}^{\text{v}}_i\boldsymbol{\beta}^\text{v}, \text{var}(\mathbf{v}_i) = \mathbf{Z}^{\text{v}}_i\mathbf{D}_{\text{v}}\mathbf{Z}_i^{\text{v}\top}+\mathbf{\Sigma}_i\right).
\end{align*}\\ \\
The integral that we want to solve in order to derive the marginal association coefficient is:
\begin{equation}
\label{ass jsm}
\begin{aligned}
E\left[y_{ik} \mid v_{ij} = a\right] 
& =\int_y y_{i k} f\left(y_{i k} \mid v_{i j}=a\right) \; d y_{ik} \\
& = \int_y y_{i k} \; \frac{f\left(y_{i k}, v_{i j}=a\right)}{f(v_{i j}=a)} \; d y_{ik} \\
& = \int_y y_{i k} \; \frac{f\left(y_{i k}, v_{i j}=a \mid \mathbf{b}_i \right) f(\mathbf{b}_i)}{f(v_{i j}=a)} \; d y_{ik} \\ 
& = \int_y y_{i k} \int_b \frac{f(y_{i k} \mid v_{i j} = a, \mathbf{b}_i)f(v_{i j}=a \mid \mathbf{b}_i) f(\mathbf{b}_i) }{f(v_{i j}=a)} \; d \mathbf{b}_i \, d y_{ik}\\ 
& = \int_y \int_b y_{i k} f\left(y_{i k}\mid v_{i j} = a, \mathbf{b}_i\right)\; \frac{ f(v_{i j}=a \mid \mathbf{b}_i) f(\mathbf{b}_i) }{f(v_{i j}=a)} \; d \mathbf{b}_i \, d y_{ik} \\ 
& = \int_b \textcolor{orange}{\int_y y_{i k} f\left(y_{i k} \mid v_{i j} = a, \mathbf{b}_i\right)} \textcolor{blue}{f\left(\mathbf{b}_i \mid v_{i j}=a\right)} \; \textcolor{orange}{d y_{ik}} \, d \mathbf{b}_i.
\end{aligned}
\end{equation}
We know the first part of the integral being the mean of $y_{ik}$ conditional on the random effects $\mathbf{b}_i$:
\begin{equation}
\label{cond mean jsm}
\textcolor{orange}{\int_y y_{i k} f\left(y_{i k} \mid v_{i j} = a, \mathbf{b}_i\right)\; d y_{ik} = g^{-1}(\eta_{ik})}.
\end{equation}
The formulation of the second part of the factorization is defined as Formula (\ref{cond b}) in Section \ref{JMM supp}.

\subsubsection{Normal case} \label{normal subsection jsm}
To measure the change in mean outcome $y_{ik}$ with a unitary increase in time-varying covariate $v_{ij}$, we need to determine the difference in expectations of the conditional distributions for a $i$-th subject:
\begin{equation*}
\label{differenceMEAN}
\begin{aligned}
& E\left[y_{ik} \mid v_{ij} =a+1\right]-E\left[y_{ik} \mid v_{ij}=a\right]= \\
& = E\left[\mathbf{x}^{\text{y}}_k\boldsymbol{\beta}^\text{y} + \boldsymbol{z}^{\text{y}}_k\mathbf{b}^{\text{y}}_i + \gamma m_{ik}) \mid v_{ij}=a+1\right]-E\left[\mathbf{x}^{\text{y}}_k\boldsymbol{\beta}^\text{y} + \boldsymbol{z}^{\text{y}}_k\mathbf{b}^{\text{y}}_i + \gamma m_{ik}) \mid v_{ij}=a\right]=\\
& = \gamma E\left[m_{ik} \mid v_{ij}=a+1\right]-\gamma E\left[m_{ik} \mid v_{ij}=a\right] ,
\end{aligned}
\end{equation*}
where $\mathbf{x}^{\text{y}}_k$ and $\mathbf{z}^{\text{y}}_k$ are the $k$-th rows of the corresponding matrices $\mathbf{X}_i^\text{y}$ and $\mathbf{Z}_i^\text{y}$, and $m_{ik}$ is the copied linear predictor of the endogenous variable for patient $i$ at a specific time point $k$. 
The only element in the linear predictor of $y_{ik}$ that depend on the values of the endogenous variable $v_{ij}$, is the linear predictor $m_{ik}$. Therefore, all the other components can be taken out of the conditional expectation. The marginal distributions of $\mathbf{v}_i$ and $\mathbf{m}_i$ are: 
$$
\begin{aligned}
&\mathbf{m}_i  \sim \mathcal{N}\left(\boldsymbol{\mu}_\text{m} =\mathbf{X}^{\text{v}}_{i} \boldsymbol{\beta}^{\text{v}}, \; \text{var}(\mathbf{m}_i) = \mathbf{Z}^{\text{v}}_i\mathbf{D}_{\text{v}}\mathbf{Z}_i^{\text{v}\top}\right), \\
&\mathbf{v}_i  \sim \mathcal{N}\left(\boldsymbol{\mu}_\text{v} = \mathbf{X}^{\text{v}}_i\boldsymbol{\beta}^\text{v}, \; \text{var}(\mathbf{v}_i) =\mathbf{Z}^{\text{v}}_i\mathbf{D}_{\text{v}}\mathbf{Z}_i^{\text{v}\top}+\mathbf{\Sigma}_i\right),
\end{aligned}
$$ thus the joint distribution is a bivariate normal, with as mean the vector of the two means $\boldsymbol{\mu}_\text{m}$ and $\boldsymbol{\mu}_\text{v}$, and as variance the matrix
$$
\left[\begin{array}{cc}
\text{var}(\mathbf{m}_i) & \text{cov}(\mathbf{m}_i, \mathbf{v}_i) \\
\text{cov}(\mathbf{m}_i, \mathbf{v}_i) & \text{var}(\mathbf{v}_i)
\end{array}\right],
$$ where $\text{cov}(\mathbf{m}_i, \mathbf{v}_i) = \mathbf{Z}^{\text{v}}_i\mathbf{D}_{\text{v}}\mathbf{Z}_i^{\text{v}\top}$.
Once again, the mean of the conditional distribution is simply derived and corresponds to:
$$
E\left(m_{ik} \mid v_{ij}=a\right)=\mu^\text{m}_{ik}+\frac{\text{cov}\left(m_{ik}, v_{ij}\right)}{\text{var}(v_{ij})}\left(a-\mu^{\text{v}}_{ij})\right).
$$
In conclusion, by replacing all the above elements in the equation we estimate the association coefficient $\beta_{joint}$:
\begin{equation}
\label{cross-sectional jsm}
\beta_{joint}= \gamma \left[\frac{\text{var}(m_{ik})}{\text{var}(v_{ij})}\right]
%\gamma\left[\frac{\mathbf{z}_k^{v\top} \mathbf{D}_v \mathbf{z}_k^{v}}{\mathbf{z}_k^{v\top} \mathbf{D}_v \mathbf{z}_k^{v}+\sigma_v^2}\right]=\gamma\left[1-\frac{\sigma_{v}^2}{\mathbf{z}_k^{v\top} \mathbf{D}_v \mathbf{z}_k^{v}+\sigma_{v}^2}\right]
\end{equation}

\section{Estimation of the association coefficient}
The procedure used to estimate the integrals in both the JMM and JSM cases is identical. When estimating the integral, three main considerations must be taken into account:
\begin{itemize}
    \item The integral cannot be computed analytically because of different types of distributions involved. Analytical computation is only possible when the outcome is a continuous variable and all distributions are normal (see Sections \ref{normal subsection jmm} and \ref{normal subsection jsm});
    \item The final forms of the integrals (\ref{ass jmm}) and (\ref{ass jsm}) involve only two distributions: the conditional mean of the outcome given the random effects, and the conditional distribution of the random effects given the endogenous variable;
    \item The models were estimated using the Bayesian estimation method INLA. The INLA output consists of univariate marginal posterior distributions for all parameters (fixed effects, random effects, scaled parameters) and hyperparameters (variances and covariances) involved, along with some summary statistics (mean, mode, quantiles, etc.). However, since the integral is defined solely by conditional distributions, the INLA output cannot be easily used to address the estimation problem.
\end{itemize}
Consequently, the Bayesian results were combined with a frequentist approach, employing Monte Carlo integration to numerically approximate the integral. As demonstrated, all the distributions involved (\ref{cond mean jmm}), (\ref{cond b}), and (\ref{cond mean jsm}) can be analytically specified. We used the mode of the univariate marginal posterior distributions as point estimates for the parameters involved $\hat{\boldsymbol{\theta}} = (\hat{\boldsymbol{\beta}^{\text{v}}}, \hat{\boldsymbol{\beta}^{\text{y}}}, \hat{\mathbf{b}}_i, \hat{\boldsymbol{\varepsilon}_i}, \hat{\textbf{D}}, \hat{\sigma})$. With this information, we were able to integrate out the random effects from the integrand and derive a numerical approximation of the association coefficient (see Figure \ref{int_method}). Following this approach, we estimated $E\left[y_{ik} \mid v_{ij} = a\right]$ and $E\left[y_{ik} \mid v_{ij} = a + 1\right]$, from which the association coefficient $\beta_{joint}$ was derived.
\begin{figure*}[!t]
    \centering
    \fbox{\includegraphics[width=1\linewidth]{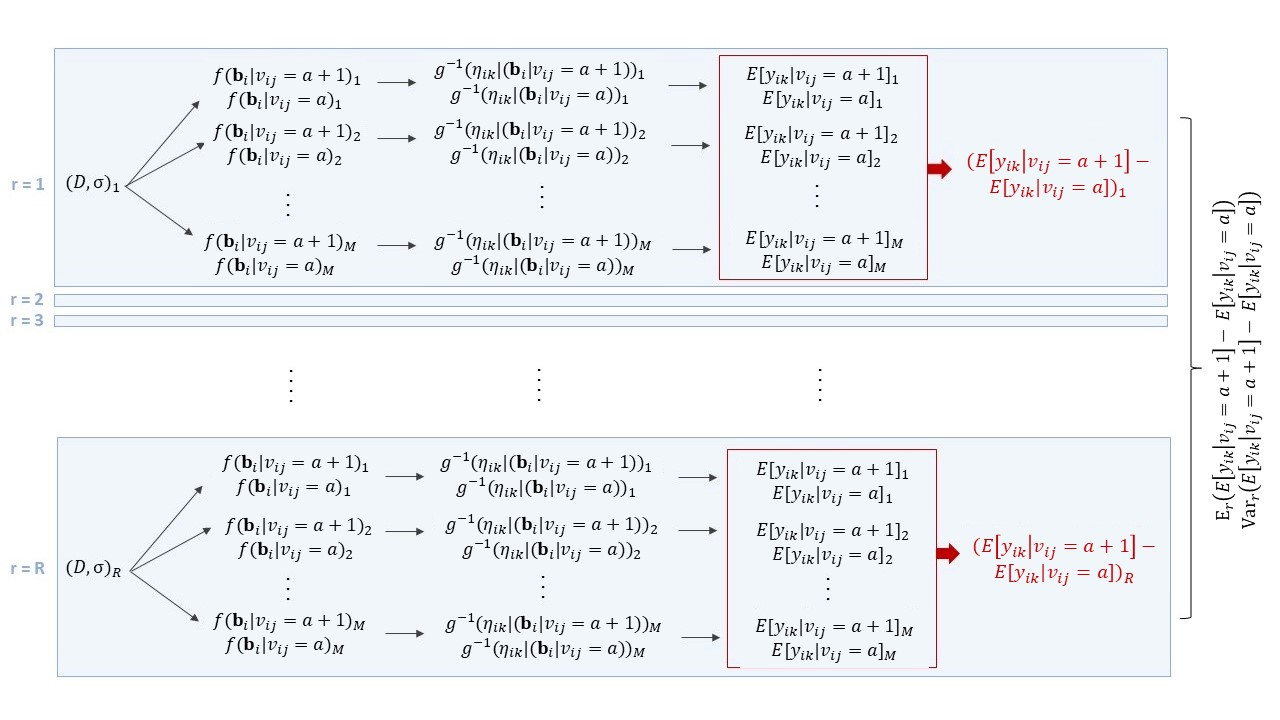}}
    \caption{Diagram of the Monte Carlo integration approximation of the association coefficient $\beta_{joint}$}\label{int_method}
\end{figure*}
\\
\\
We also wanted to derive an estimation of the uncertainty of $E\left[y_{ik} \mid v_{ij} = a\right]$. This expectation is a function of the parameters and hyperparameters $\hat{\boldsymbol{\theta}} = (\hat{\boldsymbol{\beta}^{\text{v}}}, \hat{\boldsymbol{\beta}^{\text{y}}}, \hat{\mathbf{b}}_i, \hat{\boldsymbol{\varepsilon}_i}, \hat{\textbf{D}}, \hat{\sigma})$, which are considered random variables because their values depend on the specific random samples observed.  Consequently, $E\left[y_{ik} \mid v_{ij} = a\right]$ is also a random variable, with its randomness coming from the parameters and hyperparameters. Thus, To estimate the uncertainty, we need to account for the uncertainty of $\theta$. Additionally, the variability of the parameters $(\hat{\boldsymbol{\beta}^{\text{v}}}, \hat{\boldsymbol{\beta}^{\text{y}}}, \hat{\mathbf{b}}_i, \hat{\boldsymbol{\varepsilon}_i})$ arises from the variability of the hyperparameters $\hat{\textbf{D}}, \hat{\sigma}$. Therefore, to estimate the uncertainty of $E\left[y_{ik} \mid v_{ij} = a\right]$, we must consider the potential uncertainty of the hyperparameters. To achieve this, we augment the Monte Carlo integration approximation of integral (\ref{ass jmm}) and (\ref{ass jsm}), buy adding a new layer of resampling. We sample from the approximate joint posterior distribution of the hyperparameters $\hat{\textbf{D}}, \hat{\sigma}$, which is a function available in INLA (\textit{inla.hyperpar.sample}). To see how the integration estimation is done on top on the Monte Carlo approximation refer to Figure \ref{var_method}.
\begin{figure*}[!t]
    \centering
    \fbox{\includegraphics[width=1\linewidth]{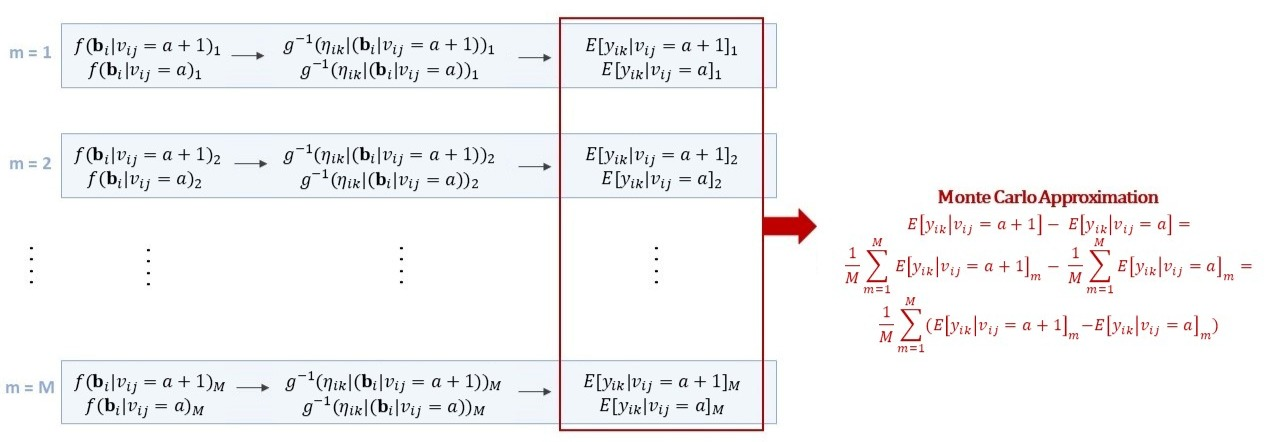}}
    \caption{Diagram of the estimation of the variance of the association coefficient $\beta_{joint}$}\label{var_method}
\end{figure*}

\section{Simulation studies}
\subsection{Default INLA prior vs informative prior}
We conducted a simulation study to assess the performance of joint models under two different specifications of the hyperprior for the precision matrix of the random effects, denoted by $\mathbf{D}^{-1}$. Data were generated following the same data generating mechanism describe in Section 5.1 of the paper. The random effects structure includes both random intercepts and random slopes, resulting in a $4 \times 4$ covariance matrix $\mathbf{D}$.
We assumed:
\begin{itemize}
    \item \textbf{Default hyperprior}:  
    \begin{center} $\mathbf{D}^{-1} \sim Wishart(11, \mathbf{R}^{-1})$ where $ \mathbf{R}^{-1} = 
    \left[\begin{array}{cccc}
    1 & 0 & 0 & 0 \\
    0 & 1 & 0 & 0 \\
    0 & 0 & 1 & 0 \\
    0 & 0 & 0 & 1 \\
    \end{array}\right]$ \end{center}
    \item \textbf{Informative hyperprior}: \\
    \begin{center}
    $\mathbf{D}^{-1} \sim Wishart(11, \mathbf{R}^{-1})$ where $ \mathbf{R}^{-1} = 
    \left[\begin{array}{cccc}
    \hat{\sigma}_1 & 0 & 0 & 0 \\
    0 & \hat{\sigma}_2& 0 & 0 \\
    0 & 0 & \hat{\sigma}_3 & 0 \\
    0 & 0 & 0 & \hat{\sigma}_4 \\
    \end{array}\right]$    
    \end{center}
     $\hat{\sigma}_1, \hat{\sigma}_2, \hat{\sigma}_3, \hat{\sigma}_4$ were estimated using maximum likelihood, by fitting separate linear mixed models (LMMs) to the response variable and to the endogenous variable.
\end{itemize}
We also investigated, in combination with the choice of hyperprior for the precision matrix, how the performance of the two joint models (JMM and JSM) is influenced by the number of available observations.\\
Figures 3-7 show the results of this simulation.

\begin{figure*}[!t]%
\centering
\includegraphics[width=0.95\linewidth]{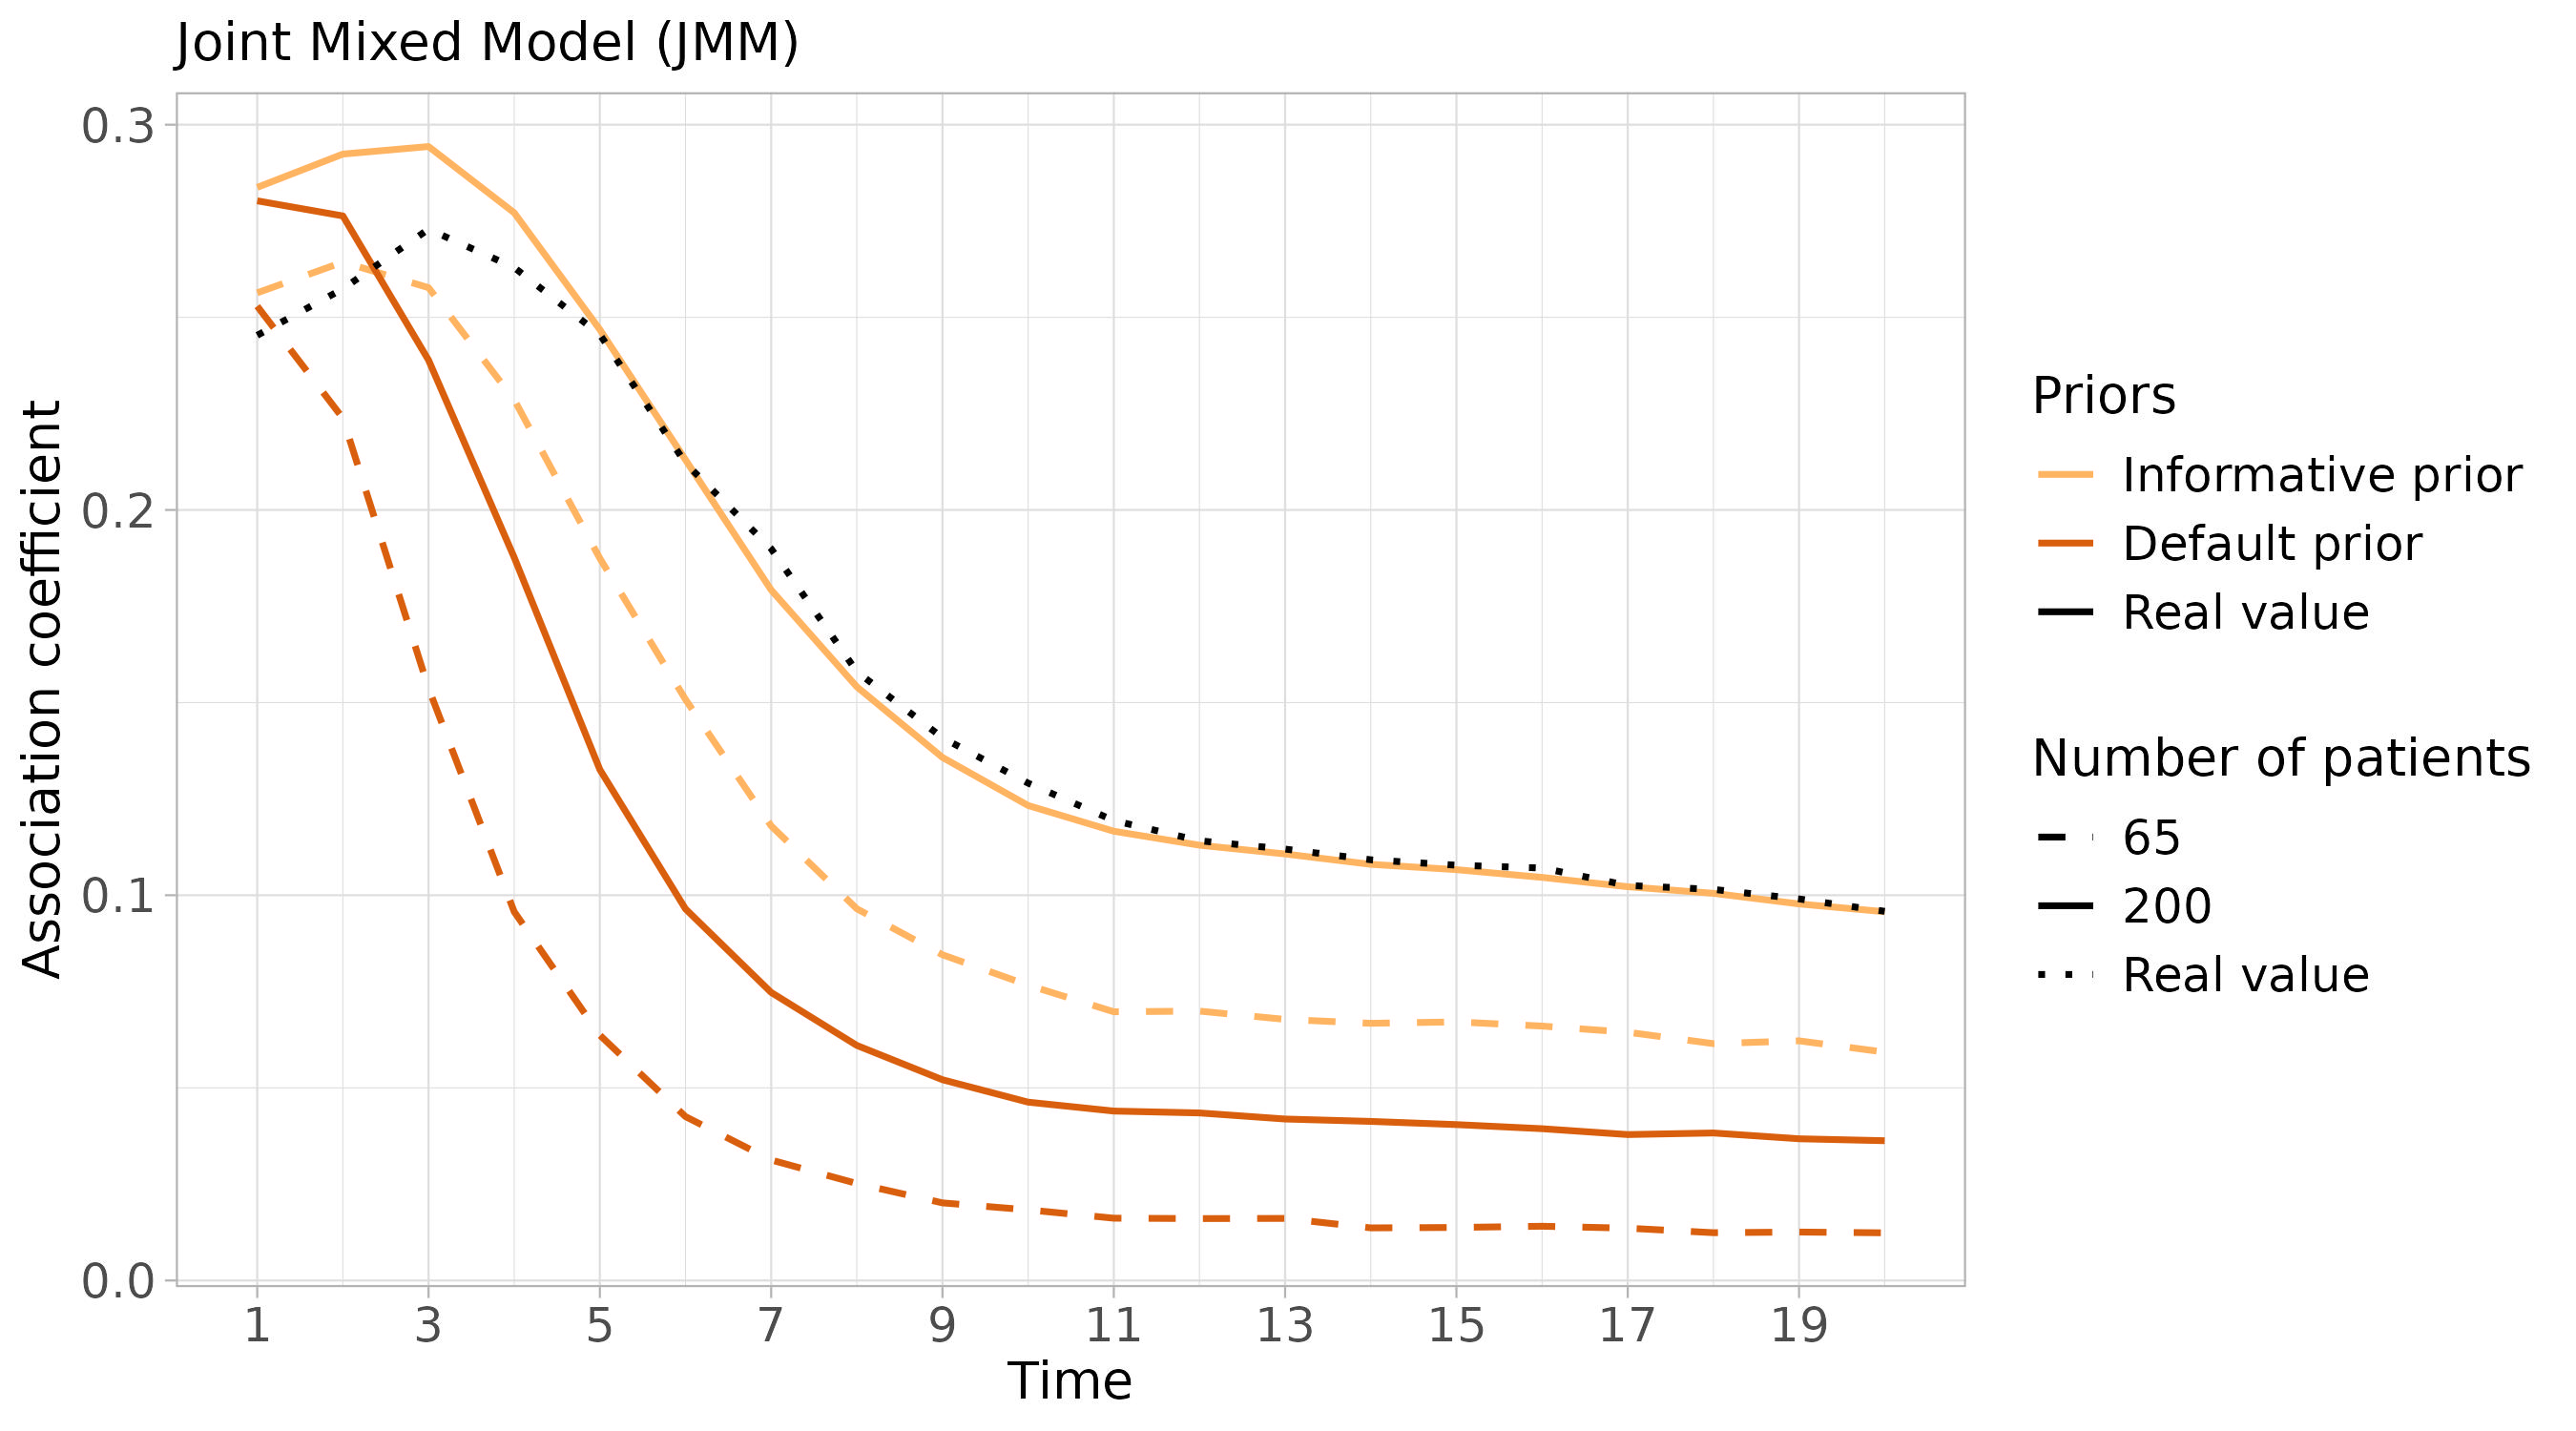}
\caption{Evaluation of the estimation of the cross-sectional association between the endogenous
covariate and the outcome in a JMM, assuming the base value $a$ set equal to the sample mean 9. The solid
lines represent the mean estimated association coefficients across B = 1000 simulations of the
JMM, assuming informative (light orange) or default (dark orange) hyperpriors for the variance-covariance matrix of the random effects. Distinction is made for sample sizes N = 65 (dashed line) and N = 200 (solid line). These are compared against the true value, indicated by the dotted black line.}
\end{figure*}

\begin{figure*}[!t]%
\centering
\includegraphics[width=0.95\linewidth]{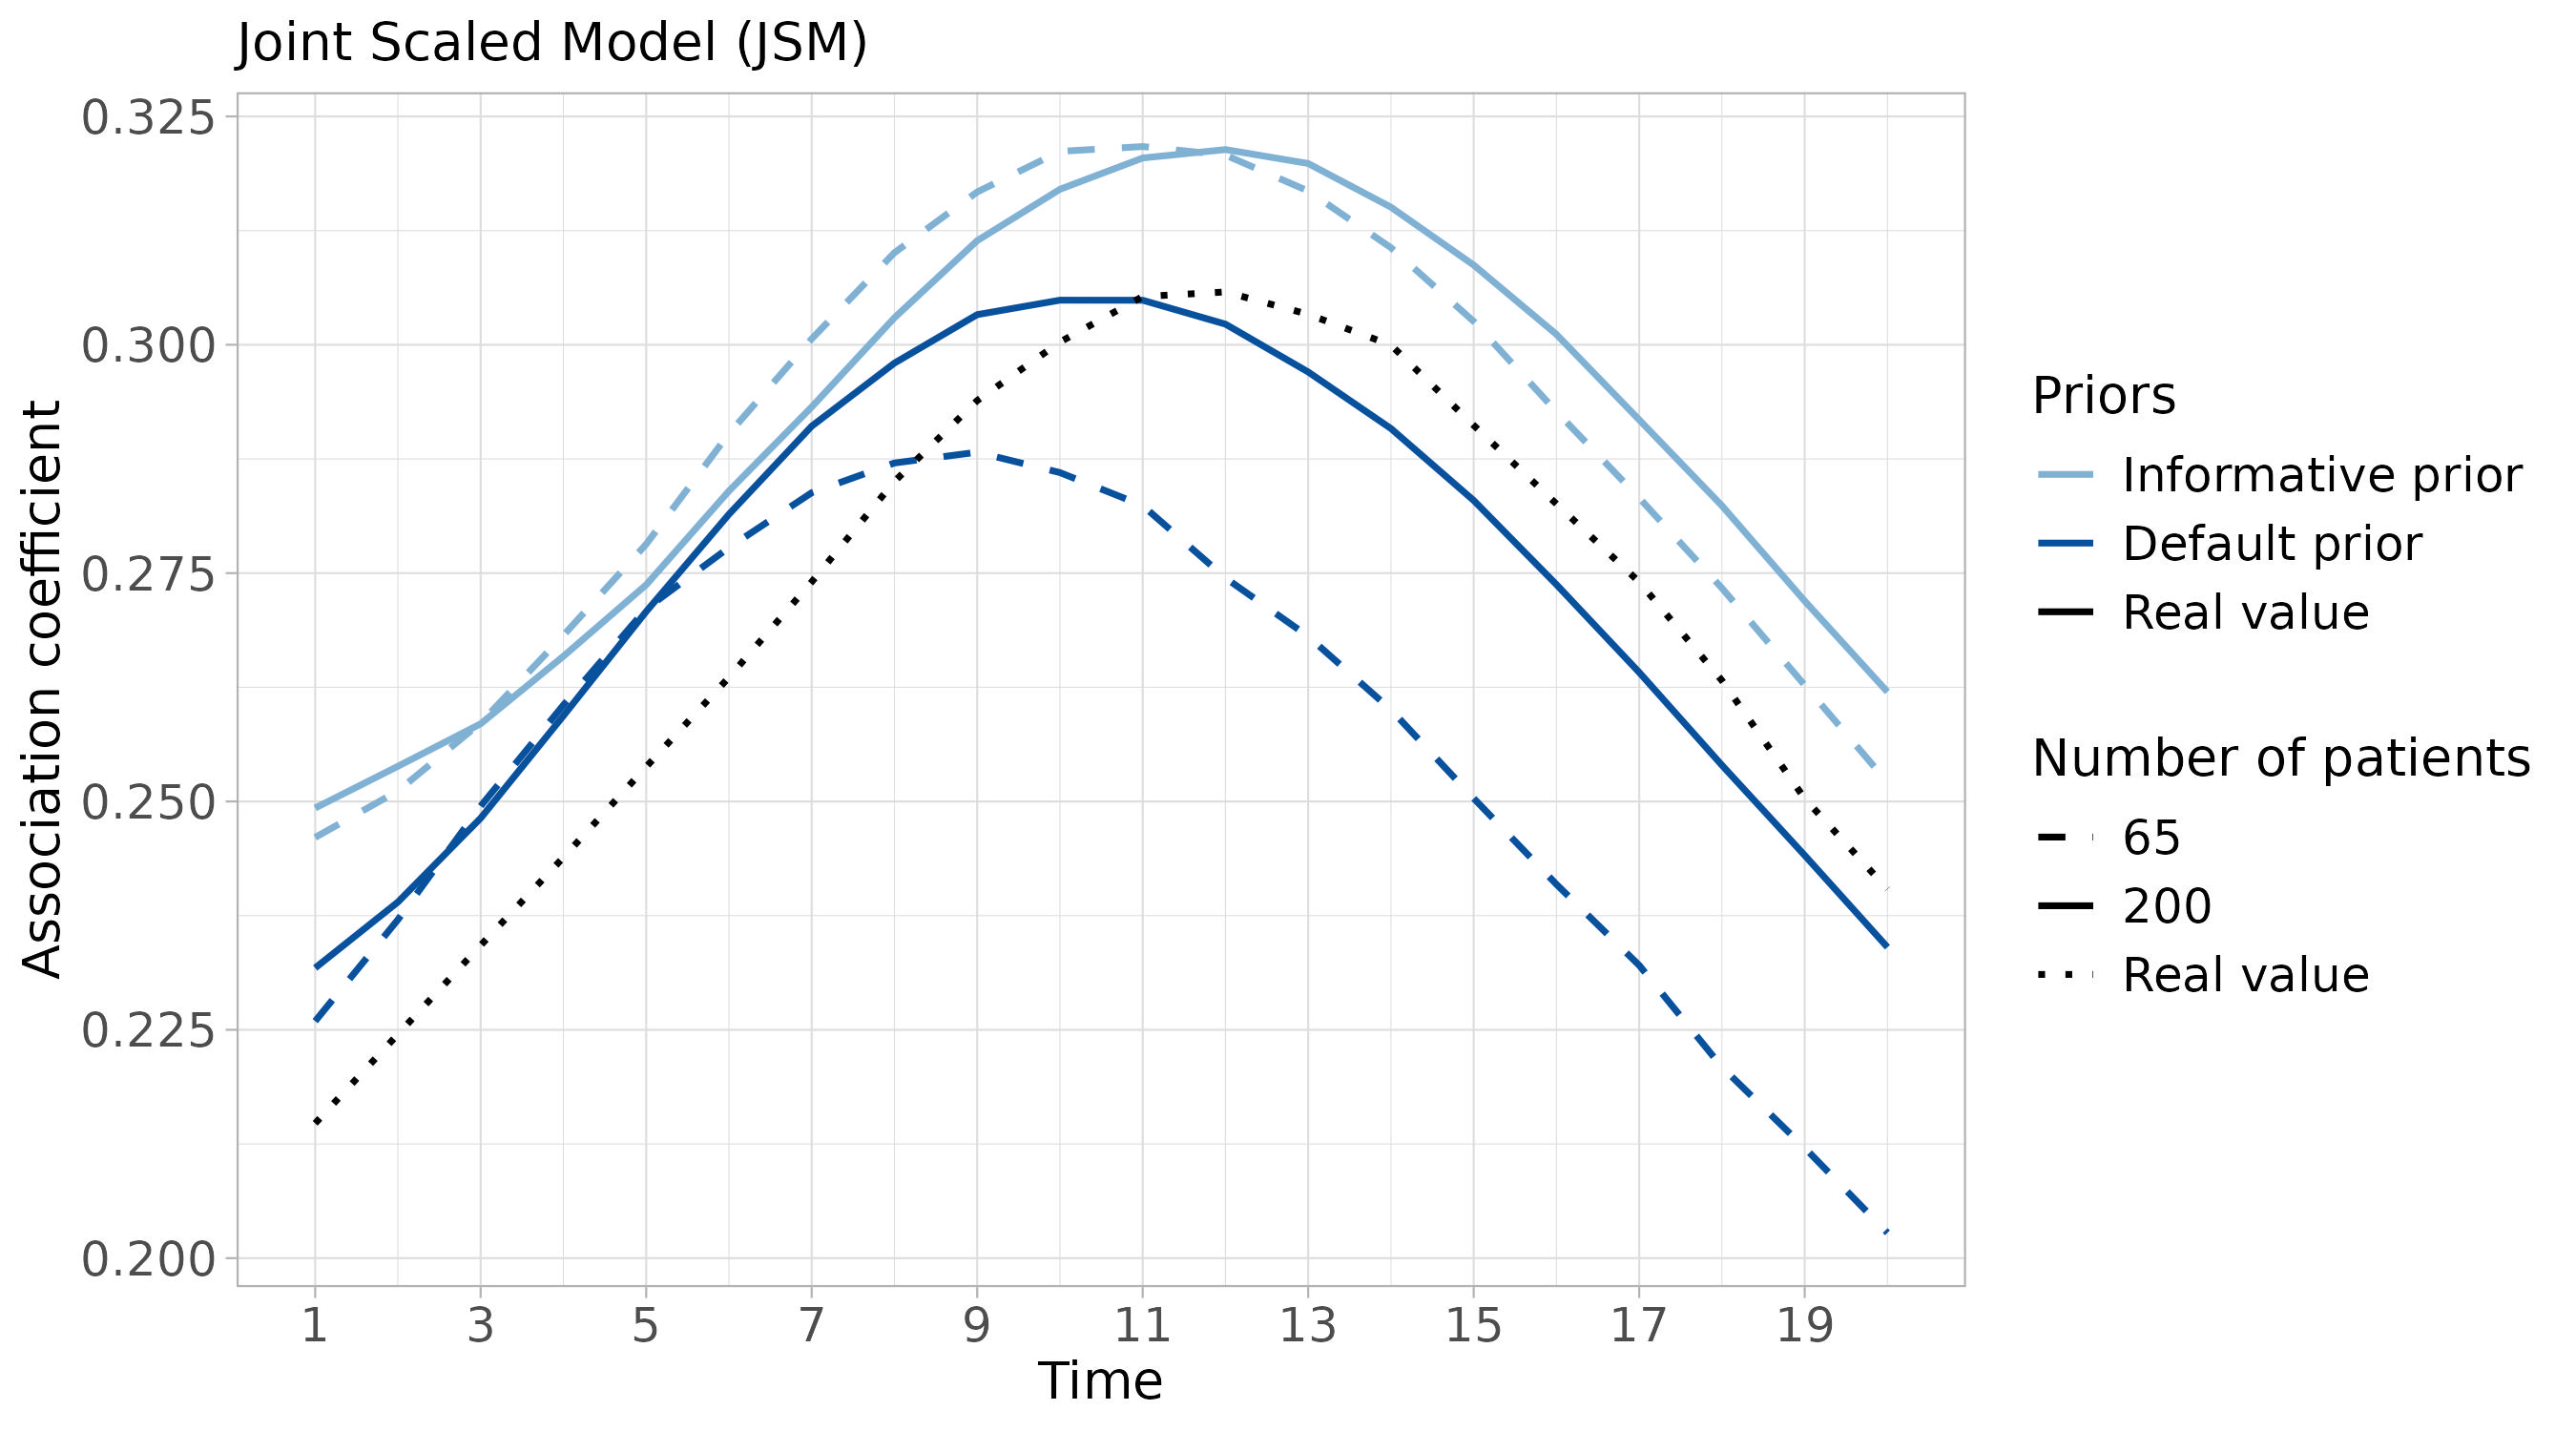}
\caption{Evaluation of the estimation of the cross-sectional association between the endogenous
covariate and the outcome in a JSM, assuming the base value $a$ set equal to the sample mean 9. The solid
lines represent the mean estimated association coefficients across B = 1000 simulations of the
JSM, assuming informative (light blue) or default (dark blue) hyperpriors for the variance-covariance matrix of the random effects. Distinction is made for sample sizes N = 65 (dashed line) and N = 200 (solid line). These are compared against the true value, indicated by the dotted black line.}
\end{figure*}

\begin{figure*}[!t]%
\centering
\includegraphics[width=0.70\linewidth]{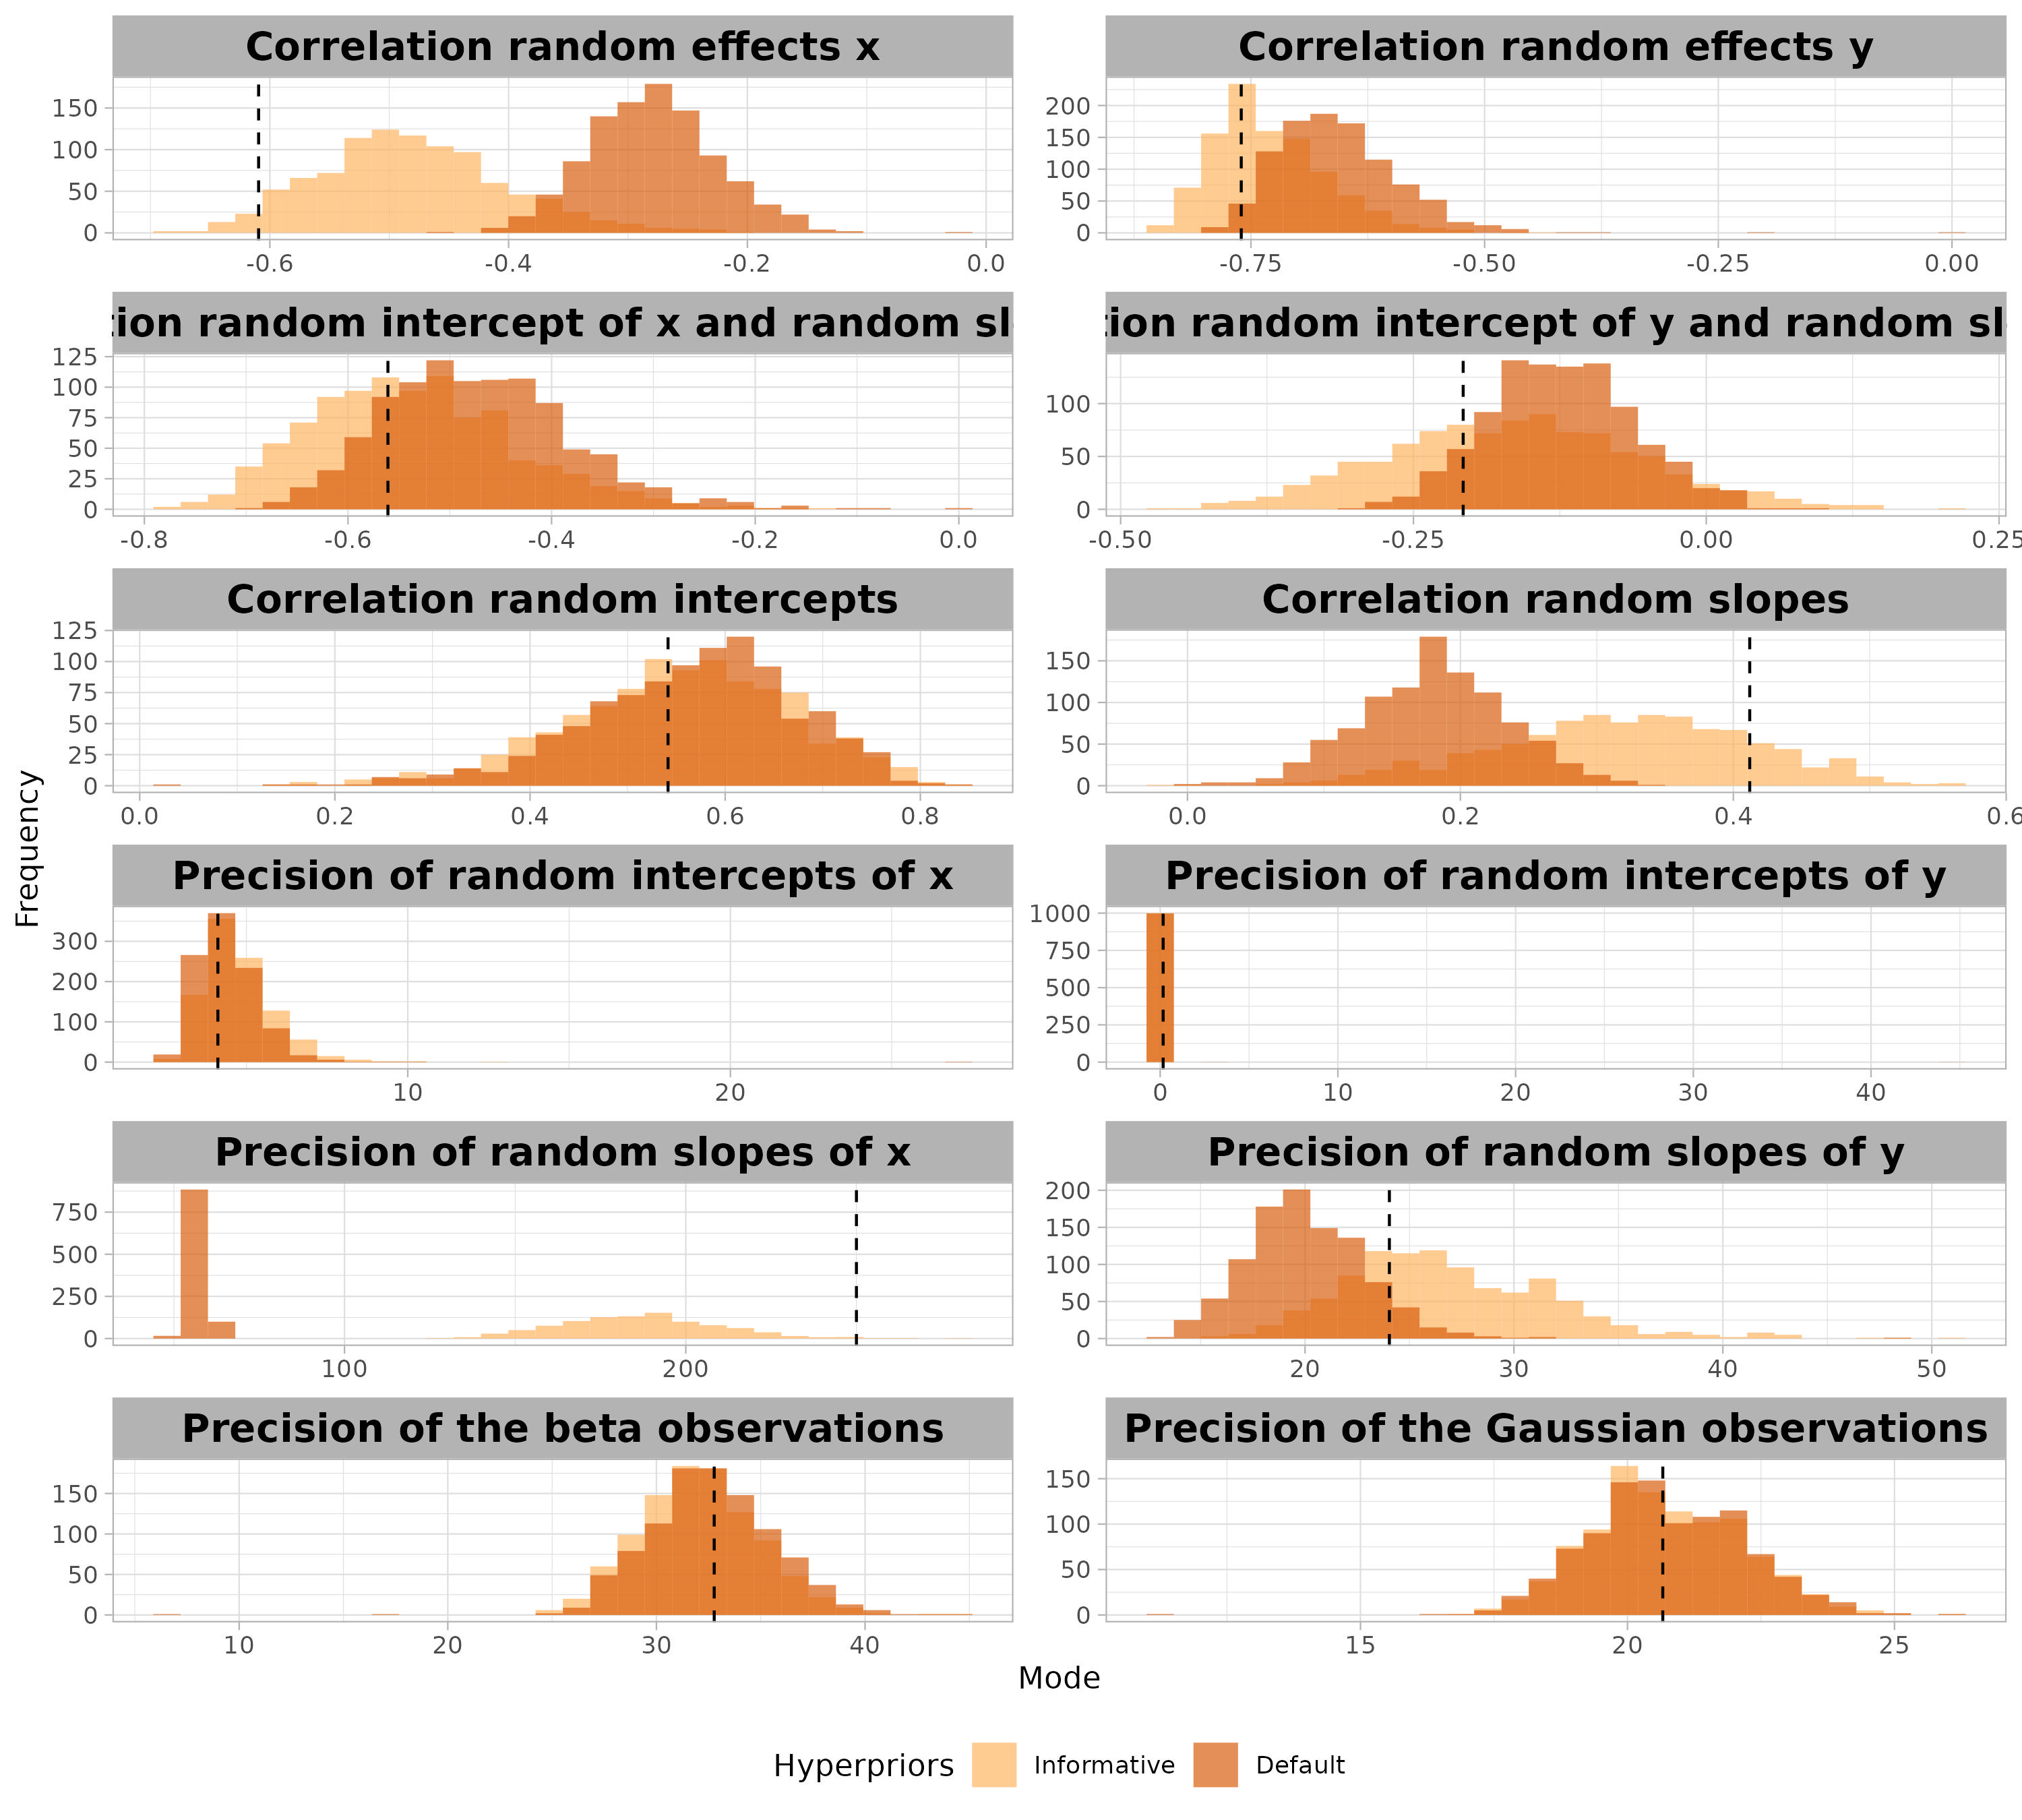}
\caption{Comparison of JMM hyperparameters posteriors modes obtain assuming informative or default hyperpriors with sample sizes $N = 65$. The histograms display the posterior modes of the hyperparameters from $B = 1000$ simulated datasets. The figure includes the variances and covariances of the random effects, the precision parameter $\phi$ of the Beta distribution governing the outcome, and the precision of the error terms $\varepsilon_i$ associated with the endogenous variable.}
\end{figure*}

\begin{figure*}[!t]%
\centering
\includegraphics[width=0.70\linewidth]{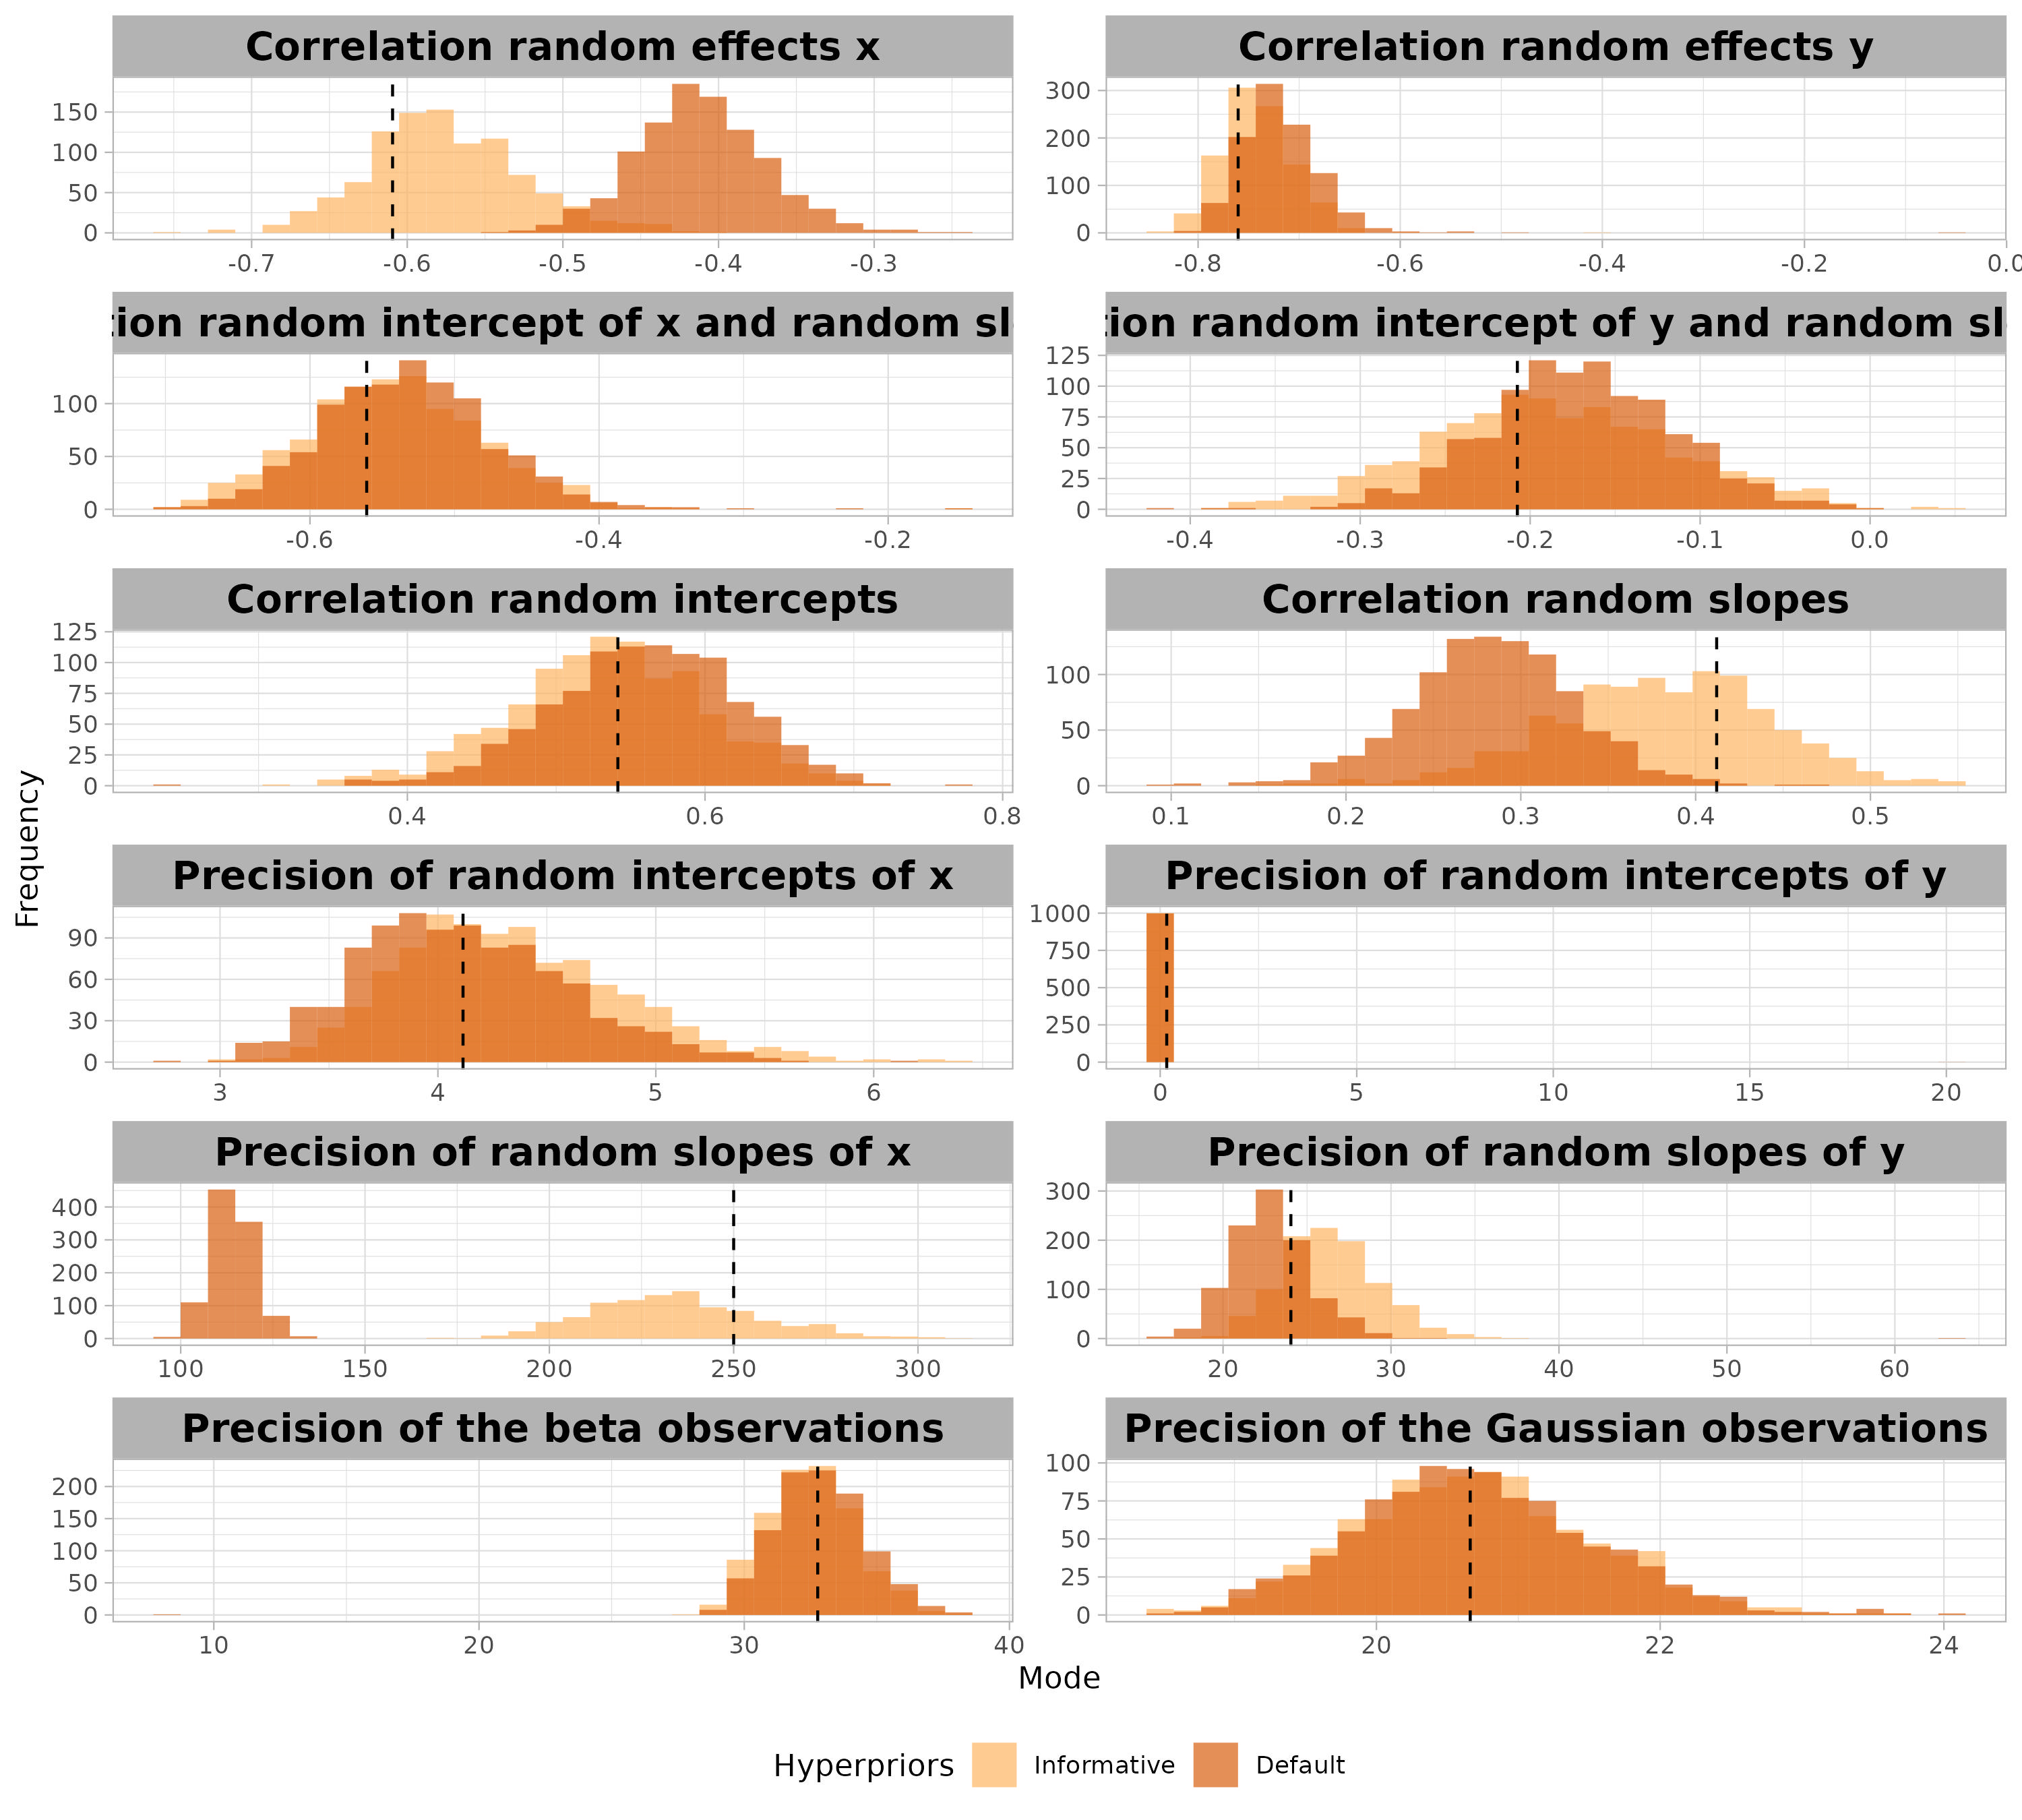}
\caption{Comparison of JMM hyperparameters posteriors modes obtain assuming informative or default hyperpriors with sample sizes $N = 200$. The histograms display the posterior modes of the hyperparameters from $B = 1000$ simulated datasets. The figure includes the variances and covariances of the random effects, the precision parameter $\phi$ of the Beta distribution governing the outcome, and the precision of the error terms $\varepsilon_i$ associated with the endogenous variable.}
\end{figure*}

\begin{figure*}[!t]%
\centering
\includegraphics[width=0.70\linewidth]{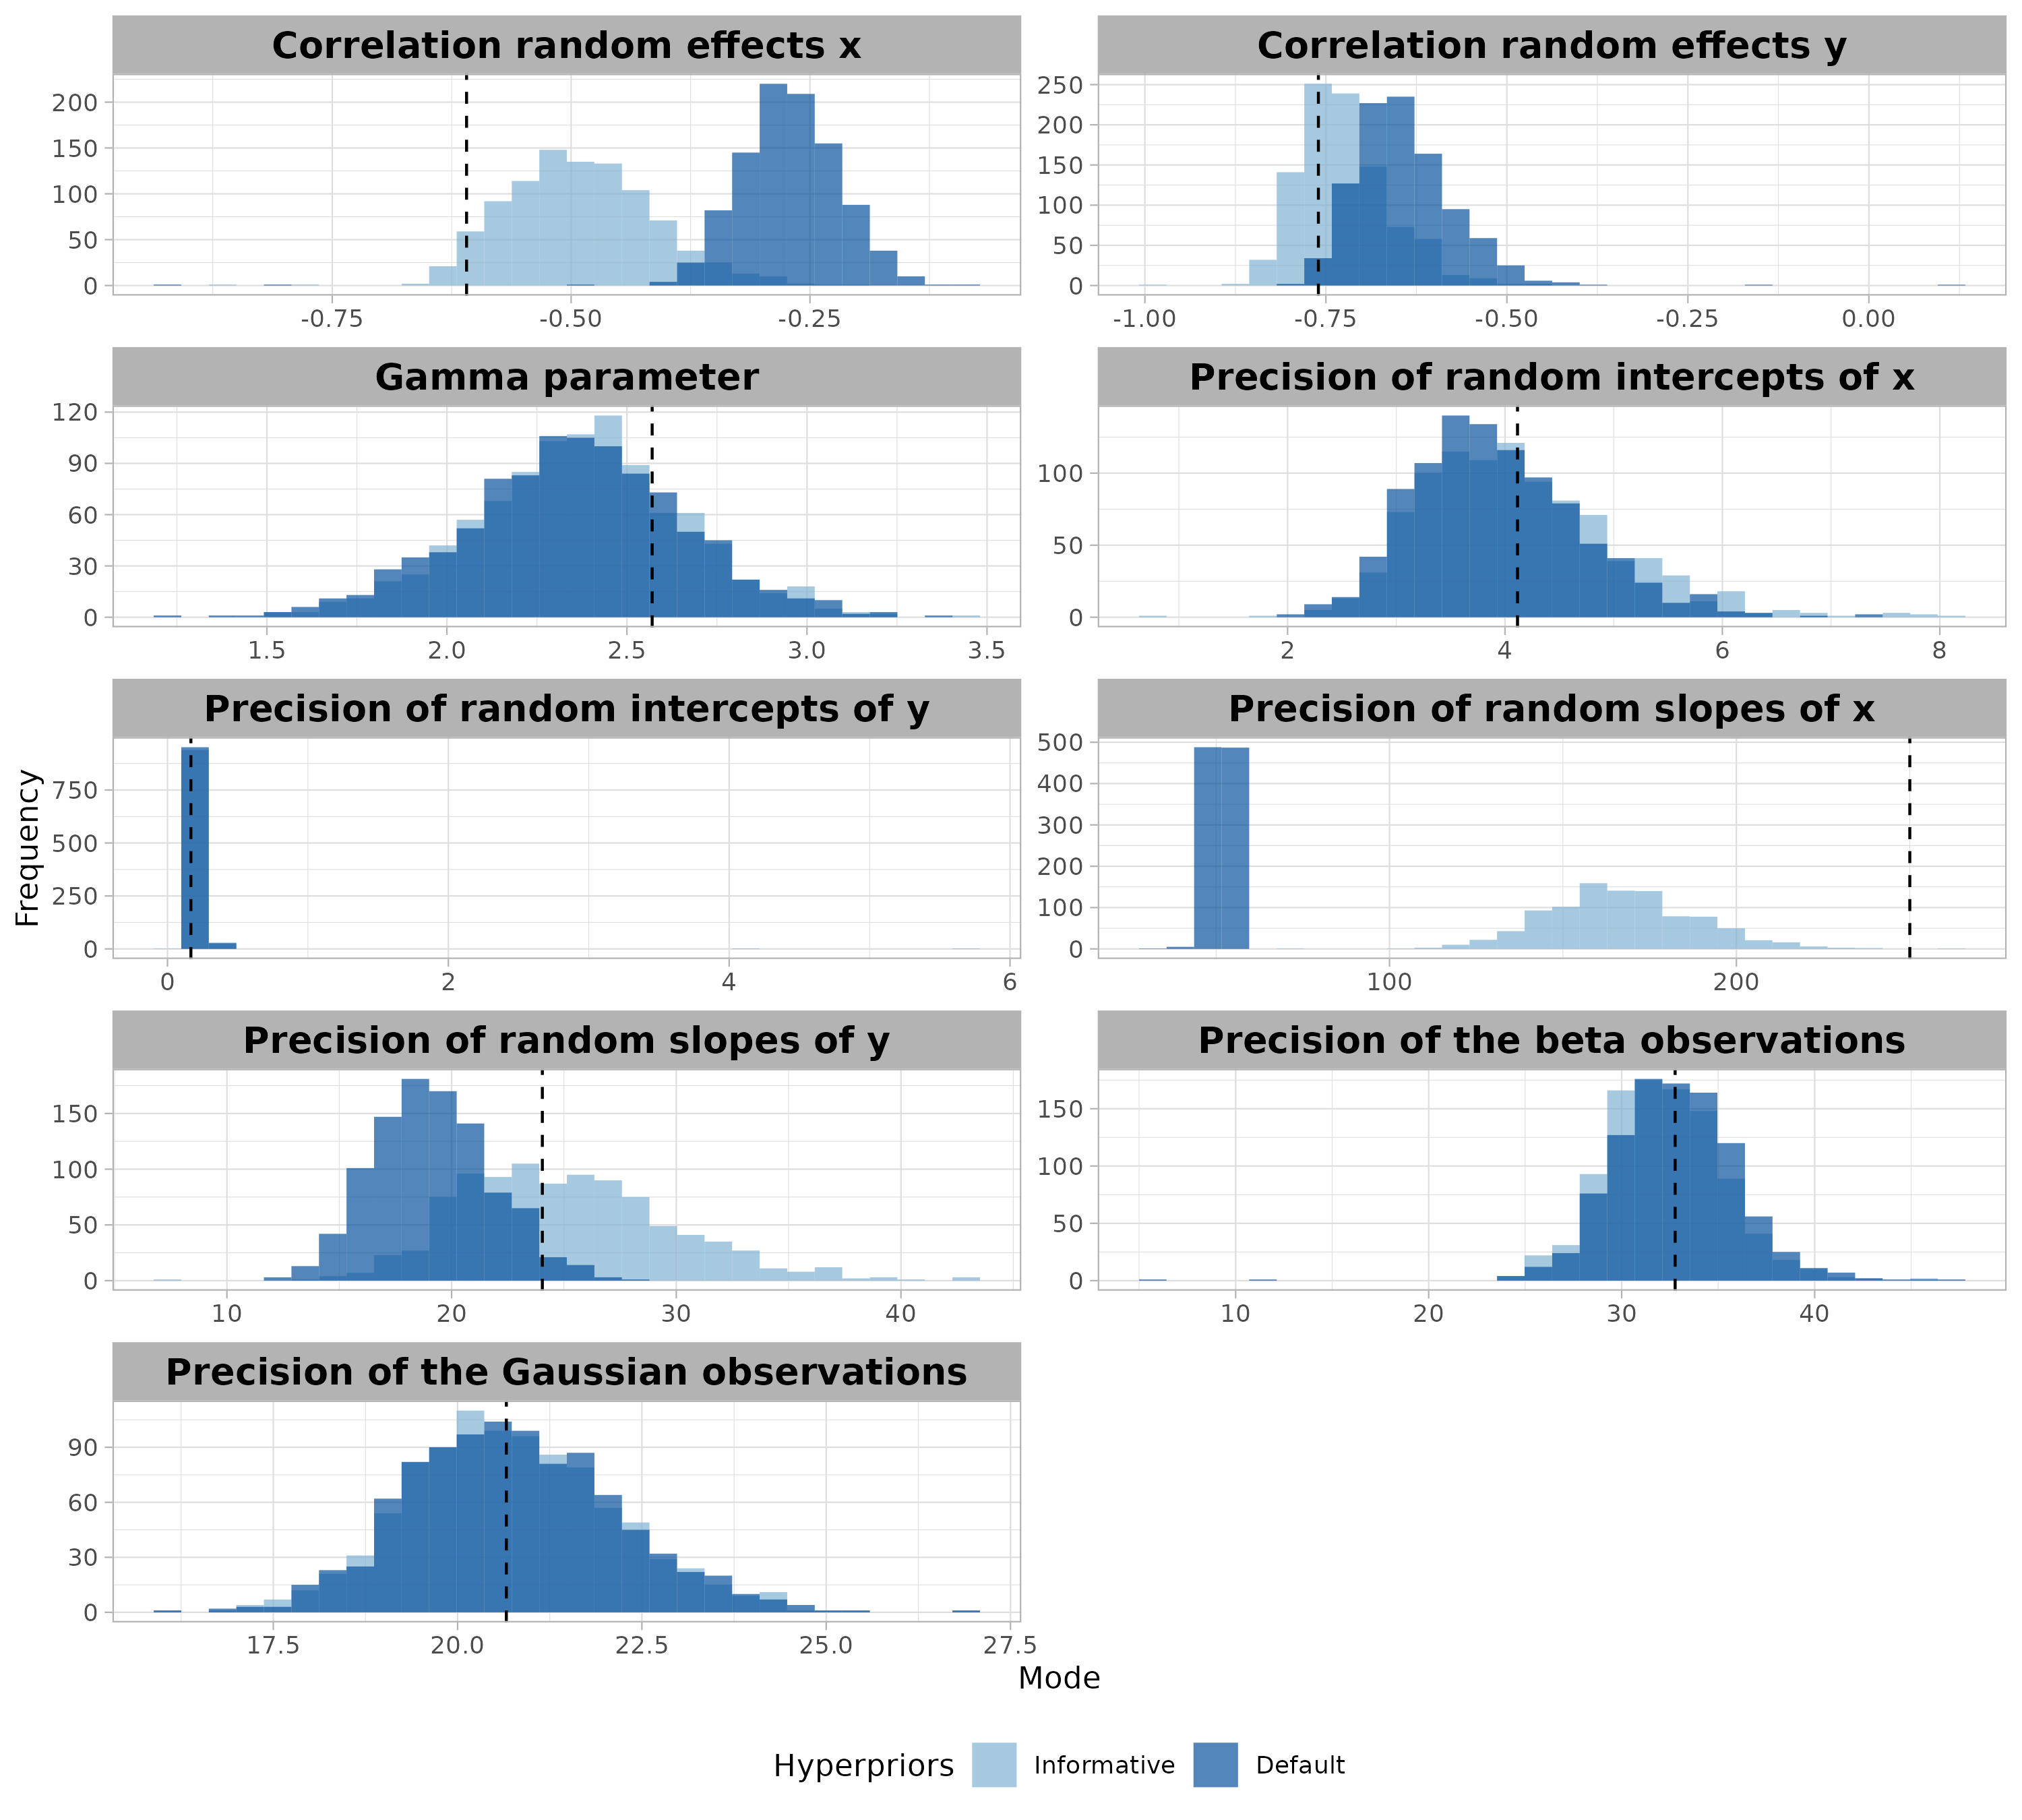}
\caption{Comparison of JSM hyperparameters posteriors modes obtain assuming informative or default hyperpriors with sample sizes $N = 65$. The histograms display the posterior modes of the hyperparameters from $B = 1000$ simulated datasets. The figure includes the variances and covariances of the random effects, the precision parameter $\phi$ of the Beta distribution governing the outcome, the precision of the error terms $\varepsilon_i$ associated with the endogenous variable, and the scaling parameter $\gamma$.}
\end{figure*}

\begin{figure*}[!t]%
\centering
\includegraphics[width=0.70\linewidth]{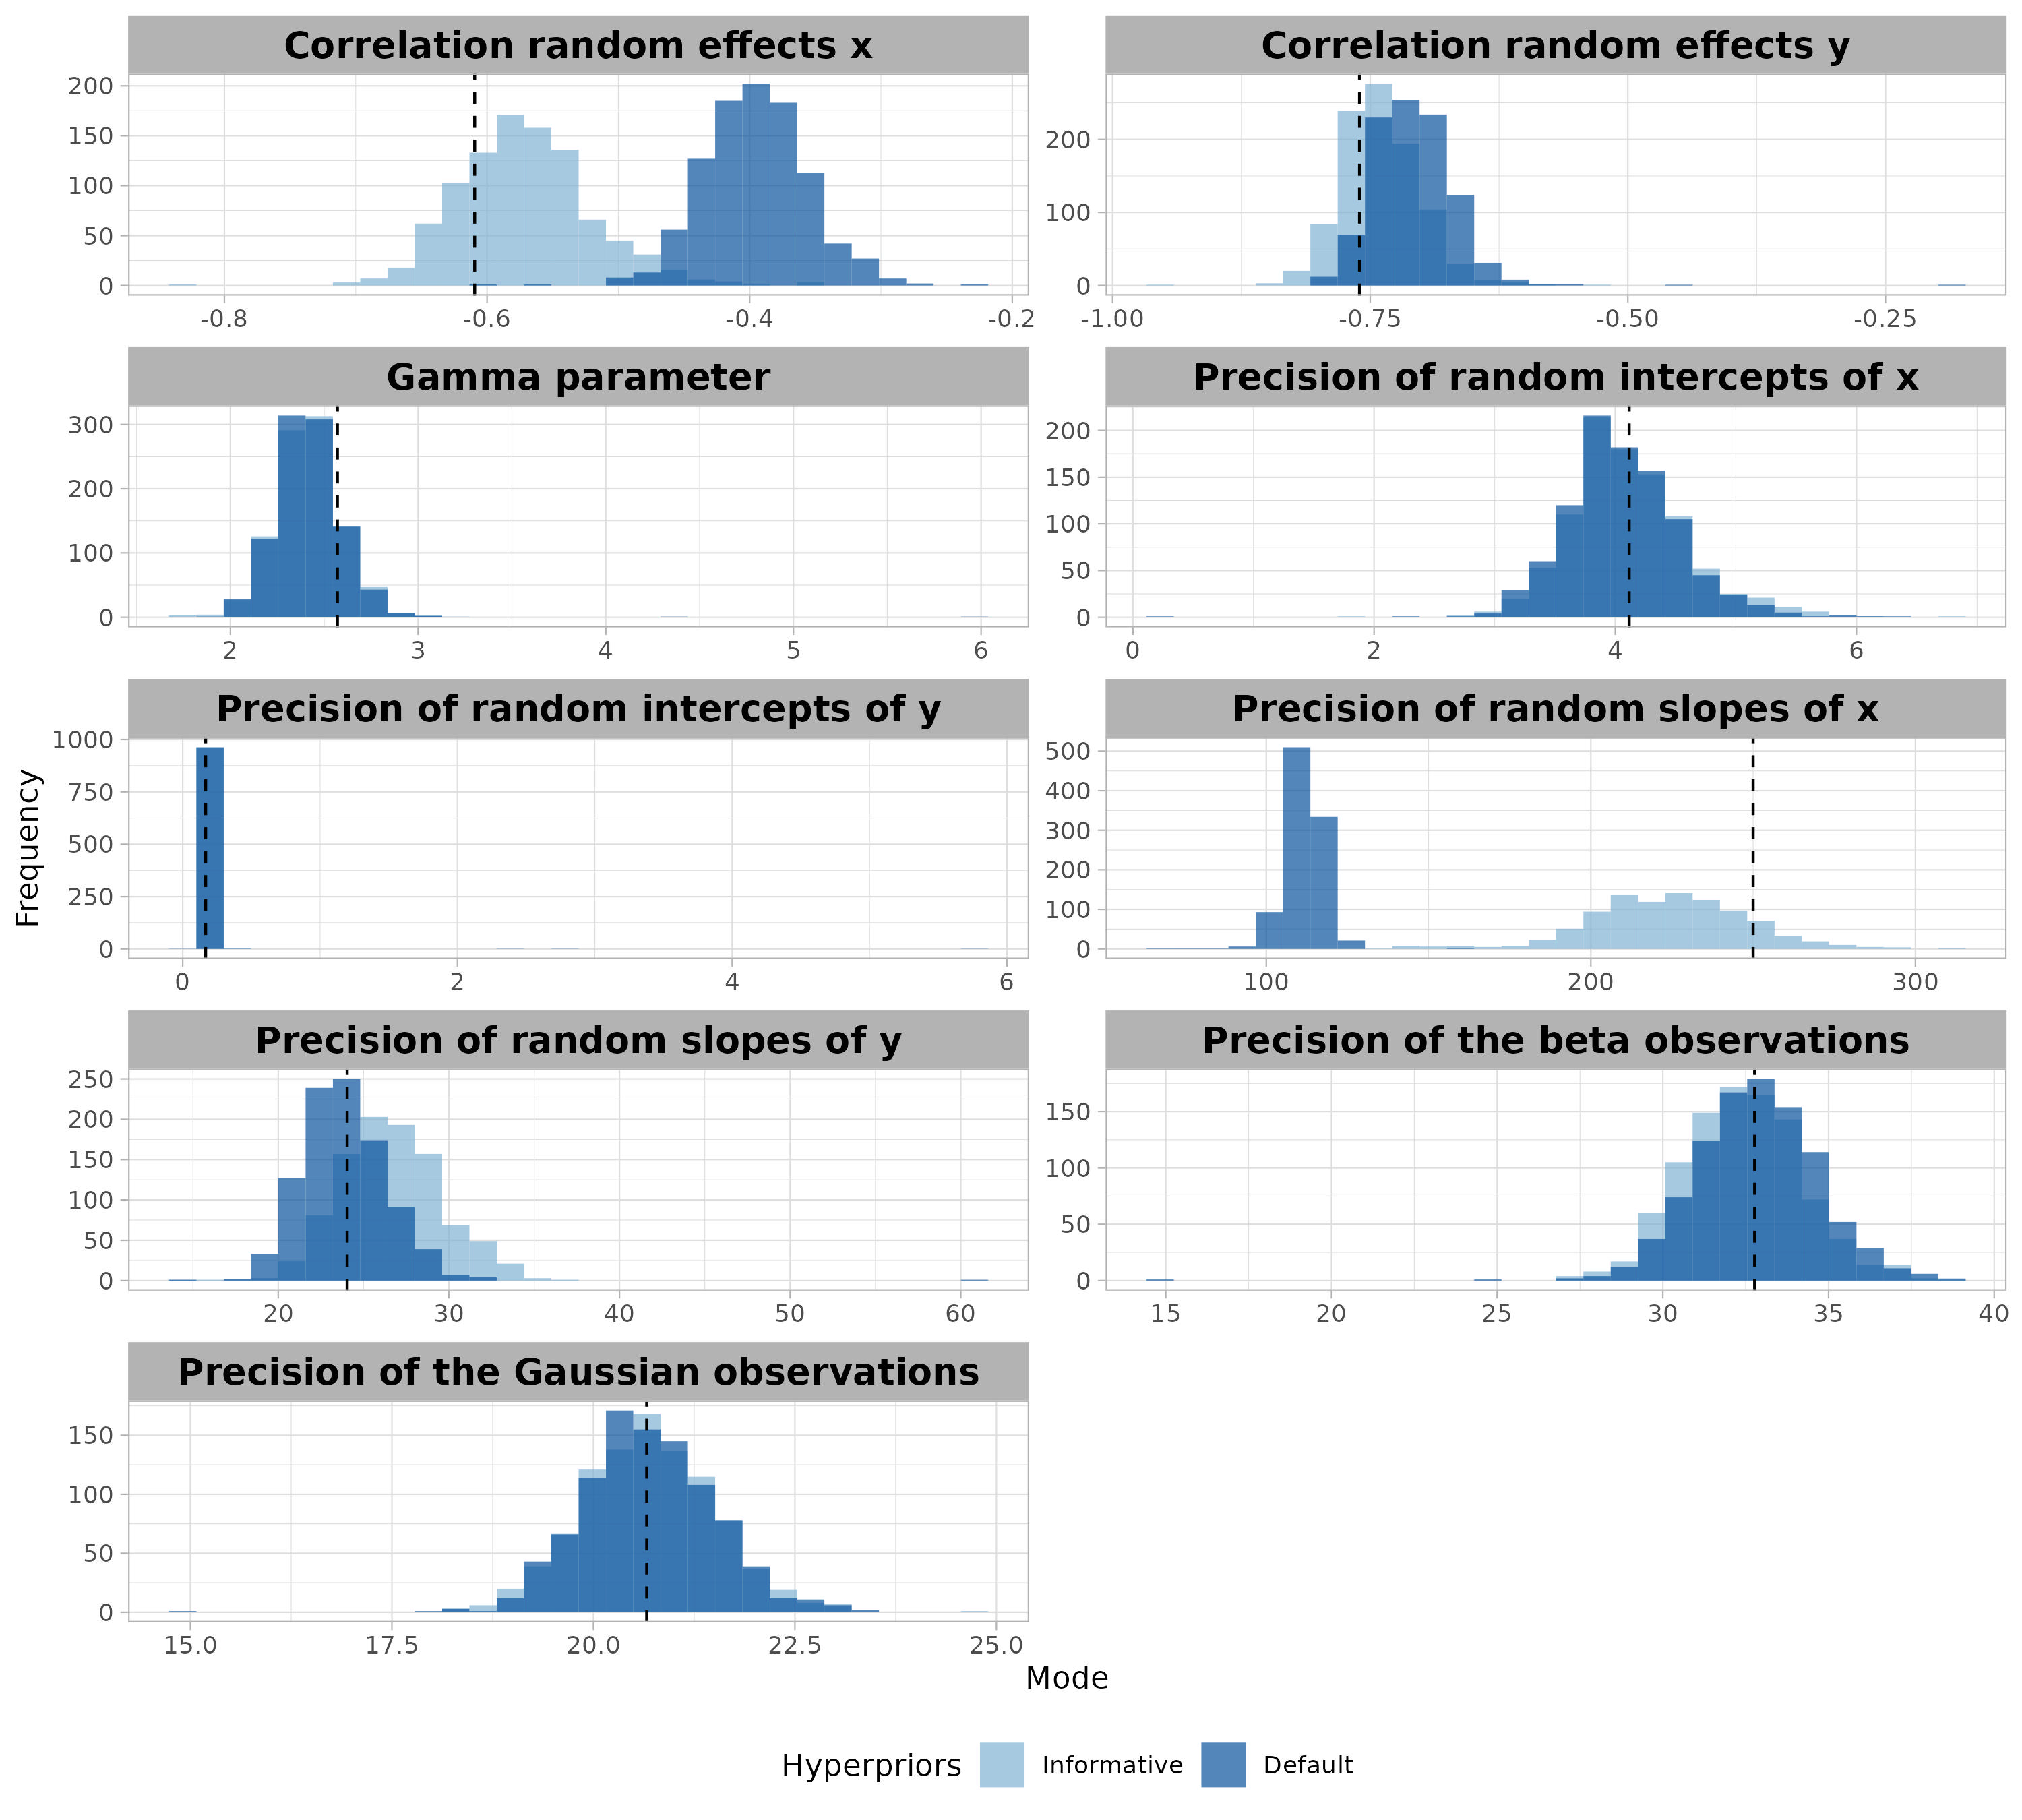}
\caption{Comparison of JSM hyperparameters posteriors modes obtain assuming informative or default hyperpriors with sample sizes $N = 200$. The histograms display the posterior modes of the hyperparameters from $B = 1000$ simulated datasets. The figure includes the variances and covariances of the random effects, the precision parameter $\phi$ of the Beta distribution governing the outcome, the precision of the error terms $\varepsilon_i$ associated with the endogenous variable, and the scaling parameter $\gamma$.}
\end{figure*}

%\subsection{Closed formula vs numerical approximation of the integral}

%\section{Application to multiple proteins}
%We conducted the same analysis shown in Section 6 of the paper for four proteins.
%\begin{figure*}[!t]%
%\centering
%\includegraphics[width=0.99\linewidth]{plot_summary (2).jpg}
%\caption{Comparison of the hyperparameters estimations among the JMM and JSM for each of the 4 proteins selected. }
%\end{figure*}

\end{document}
